# Supplementary material for: The Dataset Multiplicity Problem: How Unreliable Data Impacts Predictions
Source: arXiv:2304.10655 source file (2023-04-20)
Supplement: Supplementary file 3 [file tolerances_table.tex]

\begin{table}[t]
\small
\centering
\caption{Robustness rates for different numbers of label-flips for various classification datasets. Each entry is the percentage of test-set elements that are certifiably robust against any training-data set perturbation involving up to a the specified percentage of labels.}
\label{tab:all_data_tolerances}
\begin{tabular}{l|l|rrrrrrrrrr}\toprule
\multirow{2}{*}{Dataset} & Accuracy & \multicolumn{10}{c}{Bias level as a percentage of training dataset size}  \\
                        & \multicolumn{1}{c|}{loss} & 0.25  & 0.5 & 1.0  & 2.0  & 3.0  & 4.0 & 5.0 & 6.0 & 7.0 & 8.0 \\\midrule
\multirow{6}{*}{MNIST 1/7}  &   0 & 96.3 & 93.1 & 84.4 & 60.8 & 38.8 & 23.3 & 13.1 &  7.0 &  2.4 & 0.4 \\
                            & 0.2 & 96.7 & 93.6 & 85.8 & 63.2 & 42.5 & 27.0 & 16.1 &  9.7 & 4.6 & 1.1 \\
                            & 0.5 & 97.7 & 95.3 & 90.8 & 79.1 & 64.1 & 49.1 & 37.2 & 27.1 & 21.0 & 15.5 \\
                            & 1.0 & 98.5 & 97.3 & 94.6 & 89.8 & 84.8 & 78.0 & 69.5 & 60.8 & 51.7 & 44.9 \\
                            & 1.5 & 99.2 & 98.1 & 96.2 & 93.6 & 90.7 & 88.2 & 84.7 & 80.2 & 76.1 & 71.1 \\
                            & 2.0 & 99.2 & 98.6 & 96.9 & 94.1 & 92.0 & 89.4 & 87.0 & 83.1 & 79.6 & 76.2 \\\midrule
\multirow{6}{*}{Income}     &   0 & 81.4 & 67.8 & 50.7 & 23.3 & 12.1 &  4.8 &  1.7 & 0.7 & 0 & 0  \\
                            & 0.2 & 83.5 & 71.4 & 54.7 & 27.6 & 12.9 &  6.2 &  2.0 &   1.3 &  0& 0 \\
                            & 0.5 & 87.6 & 75.6 & 59.3 & 36.0 & 17.5 &  9.2 &  3.6 &  1.6 &  1.1 & 0 \\
                            & 1.0 & 94.1 & 86.7 & 70.6 & 51.4 & 35.9 & 24.0 & 16.9 &  9.5 &  6.0 &  2.9 \\
                            & 1.5 & 94.1 & 89.3 & 78.4 & 57.6 & 43.2 & 32.5 & 24.0 & 16.4 & 10.9 &  7.3 \\
                            & 2.0 & 94.2 & 89.6 & 81.0 & 58.9 & 45.7 & 34.4 & 25.7 & 18.5 & 11.7 &  9.0 \\\midrule
\multirow{6}{*}{HMDA}     &   TODO &  &  &  & 46.6 & 31.9 & 17.9 &  6.7 &  0.4 & 0 & 0 \\
                            &  & & 85.4 & 73.6 & 46.9 & 32.5 & 18.5 &  7.3 &  0.3 & 0 & 0 \\
                            &  &  & 86.2 & 74.3 & 51.7 & 37.8 & 26.0 & 14.4 &  4.2 & 0 & 0 \\
                            &  & & 88.5 & 74.3 & 56.7 & 42.5 & 27.1 & 19.1 & 10.8 & 0.8 & 0 \\
                            & 1.5 & 95.7 & 89.8 & 73.1 & 58.1 & 43.9 & 30.5 & 20.7 & 13.4 & 3.4 &. 0 \\
                            & 2.0 & 94.5 & 89.4 & 76.4 & 61.1 & 48.3 & 37.0 & 30.3 & 19.5 & 13.5 & 3.7 \\

\bottomrule   
\end{tabular}
\end{table}
